# Supplementary material for: Simulating Opinion Dynamics with Networks of LLM-based Agents
Source: arXiv:2311.09618 source file (2024-04-01)
Supplement: Supplementary file 1 [file result_other_topics.tex]

\section{Results of Other Topics}\label{app:result_other_topics}

In this section, we report the results of opinion evolution and final opinion state analysis with agents using both the cumulative memory as well as the reflective memory, for the topics of flat earth (see Figure \ref{fig:flat_earth_cumulative} and \ref{fig:flat_earth_reflective}), co-existence of humans and the T-Rex (see Figure \ref{fig:trex_humans_cumulative} and \ref{fig:trex_humans_reflective}), talking to the dead (see Figure \ref{fig:talking_to_dead_cumulative} and \ref{fig:talking_to_dead_reflective}), and future prediction by reading palm characteristics (see Figure \ref{fig:future_predictions_cumulative} and \ref{fig:future_predictions_reflective}).

\begin{figure*}[htb!] 
\centering
\includegraphics[width=0.99\linewidth]{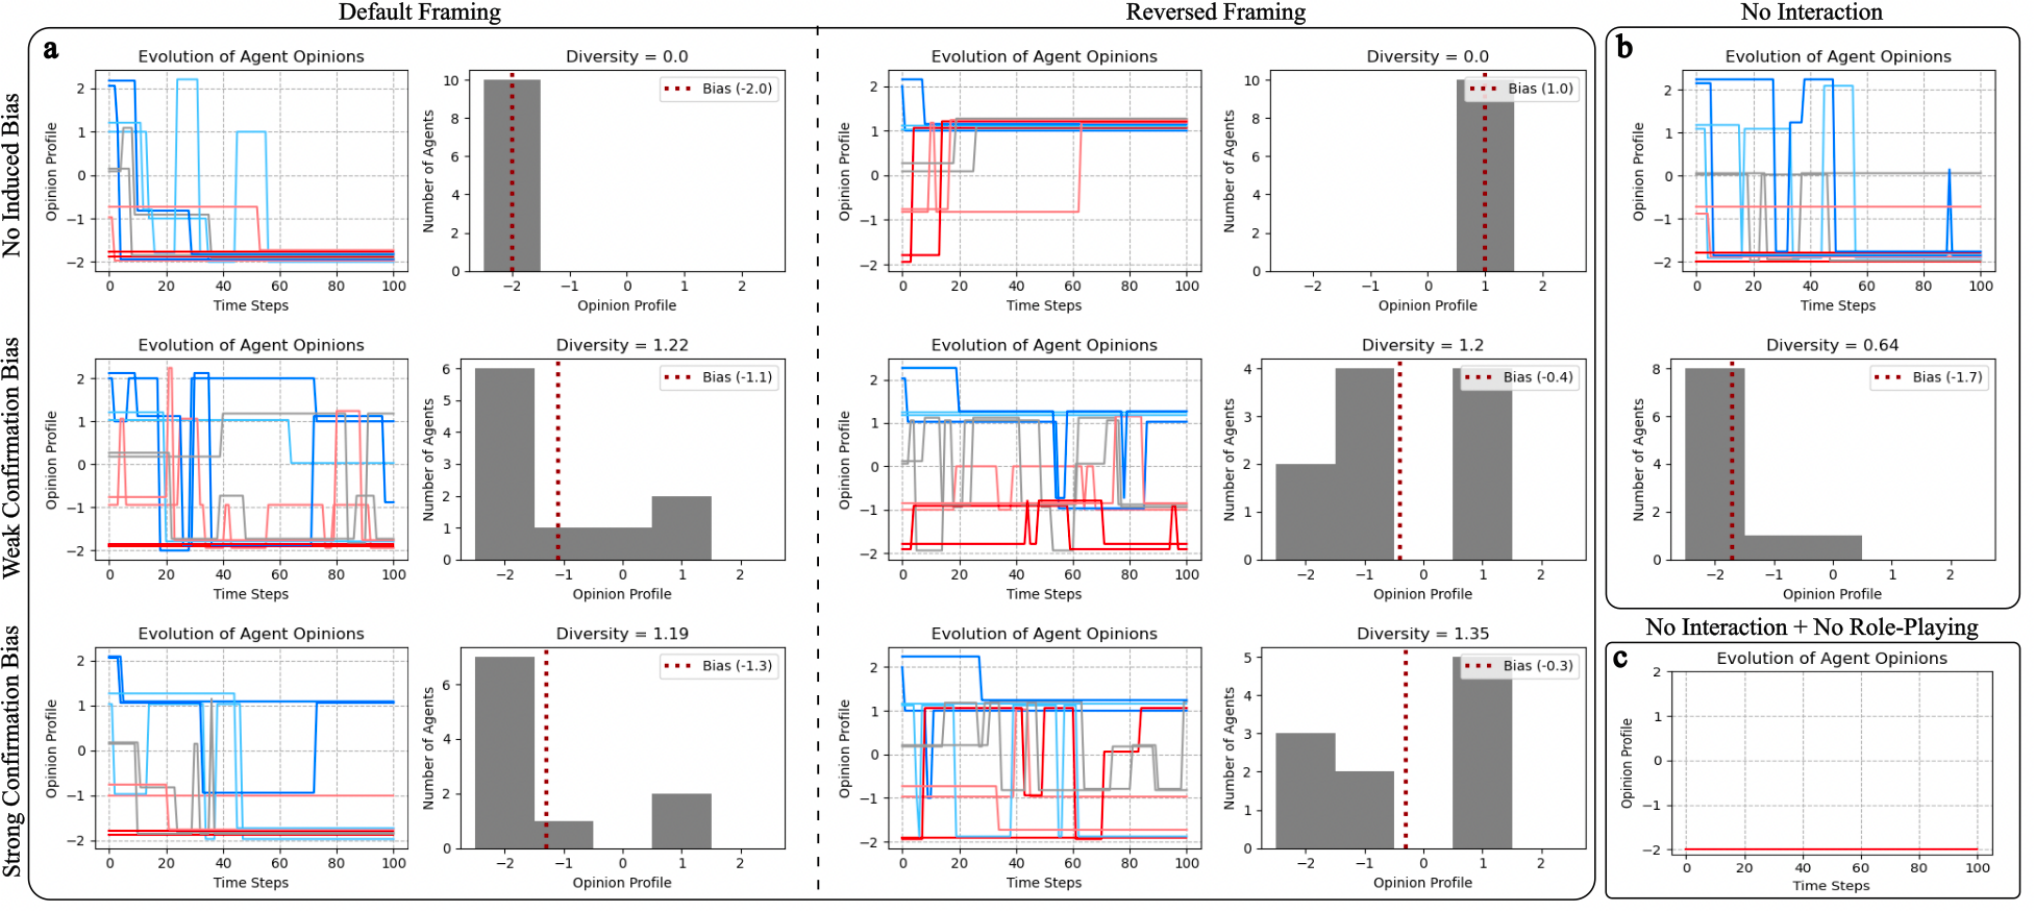}
\vspace{-2mm}
\caption{\textbf{Cumulative Memory:} Opinion trajectories $\langle o_i \rangle$ of LLM agents  and the final opinion distribution $F_{o}^T$ for the topic of Flat Earth across (a) different framings and cognitive biases, compared to baselines with (b) no interaction, and (c) no role-playing.}
\label{fig:flat_earth_cumulative}
\vspace{-4mm}
\end{figure*}
\begin{figure*}[tb!] 
\centering
\includegraphics[width=0.99\linewidth]{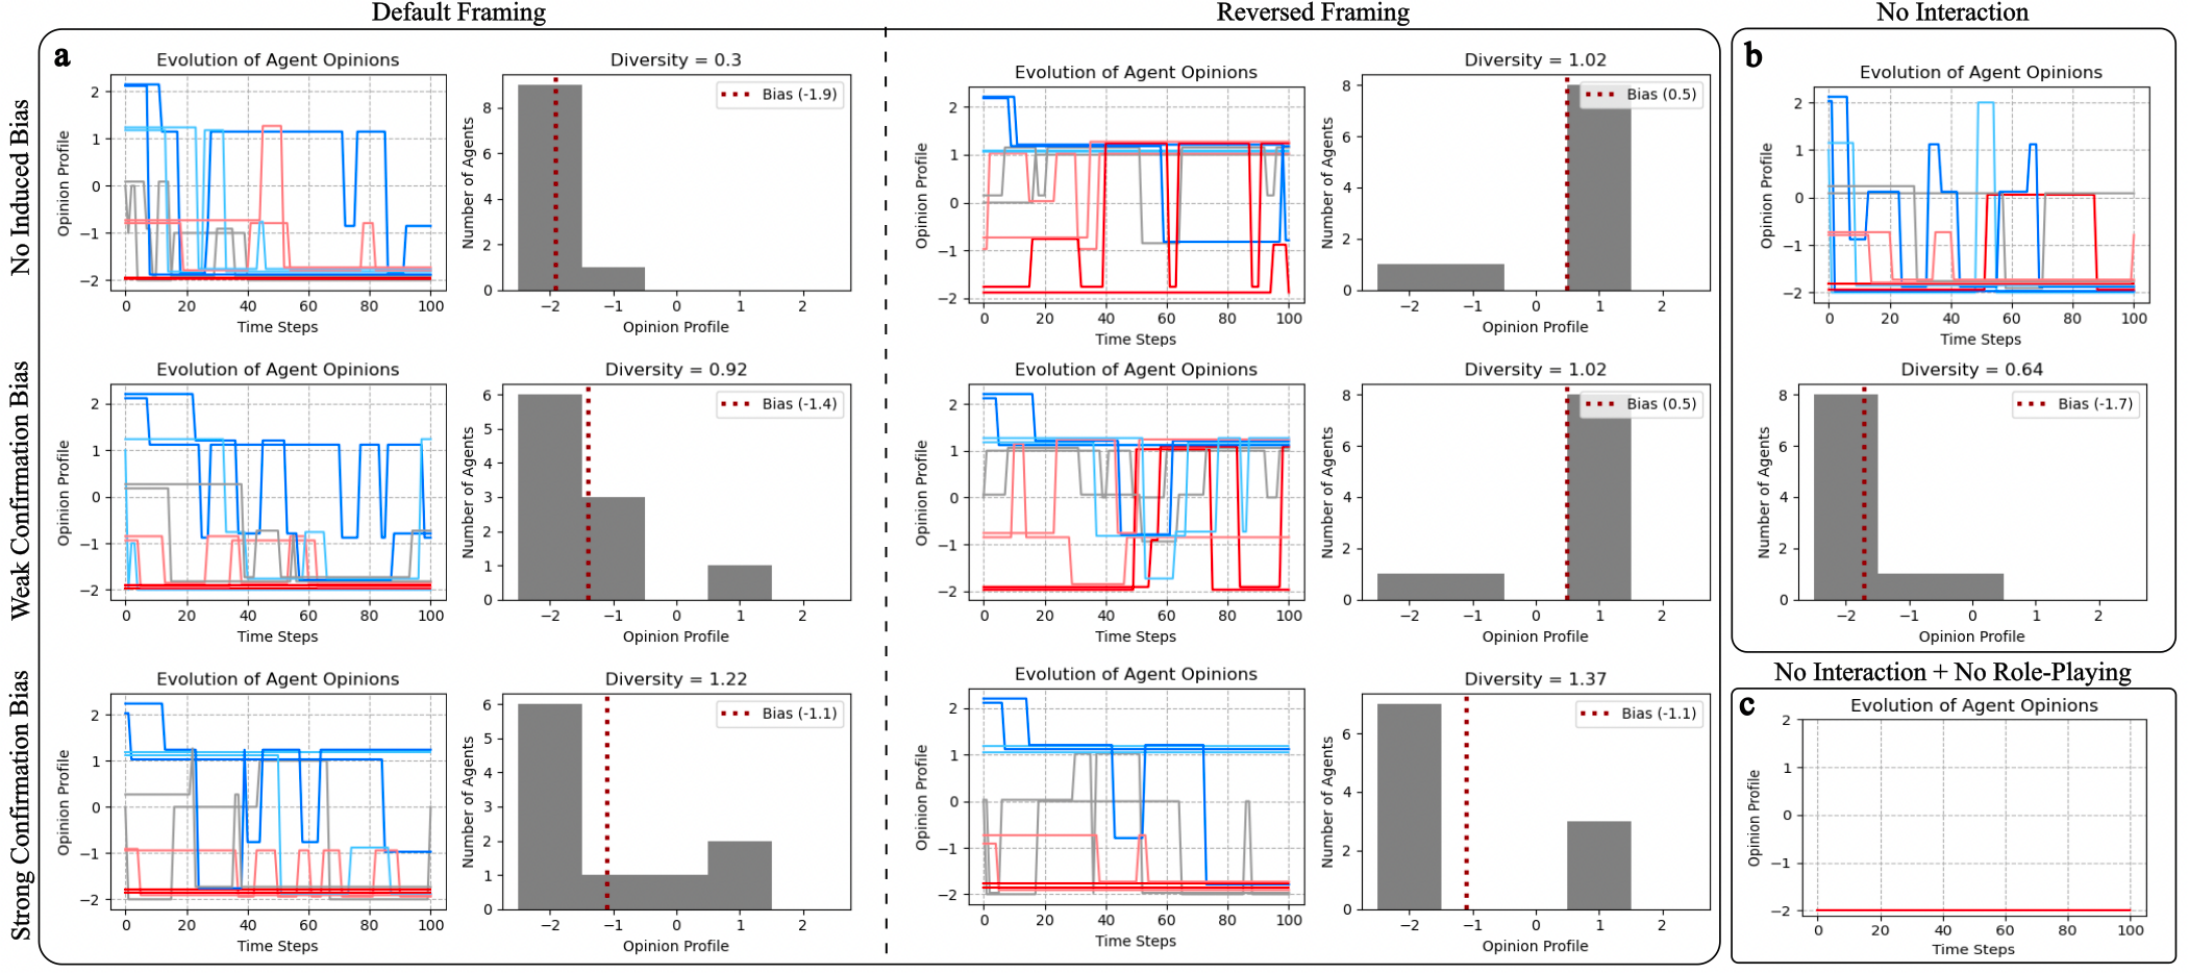}
\vspace{-2mm}
\caption{\textbf{Reflective Memory:} Opinion trajectories $\langle o_i \rangle$ of LLM agents  and the final opinion distribution $F_{o}^T$ for the topic of Flat Earth across (a) different framings and cognitive biases, compared to baselines with (b) no interaction, and (c) no role-playing.}
\label{fig:flat_earth_reflective}
\vspace{-4mm}
\end{figure*}

\begin{figure*}[htb!] 
\centering
\includegraphics[width=0.99\linewidth]{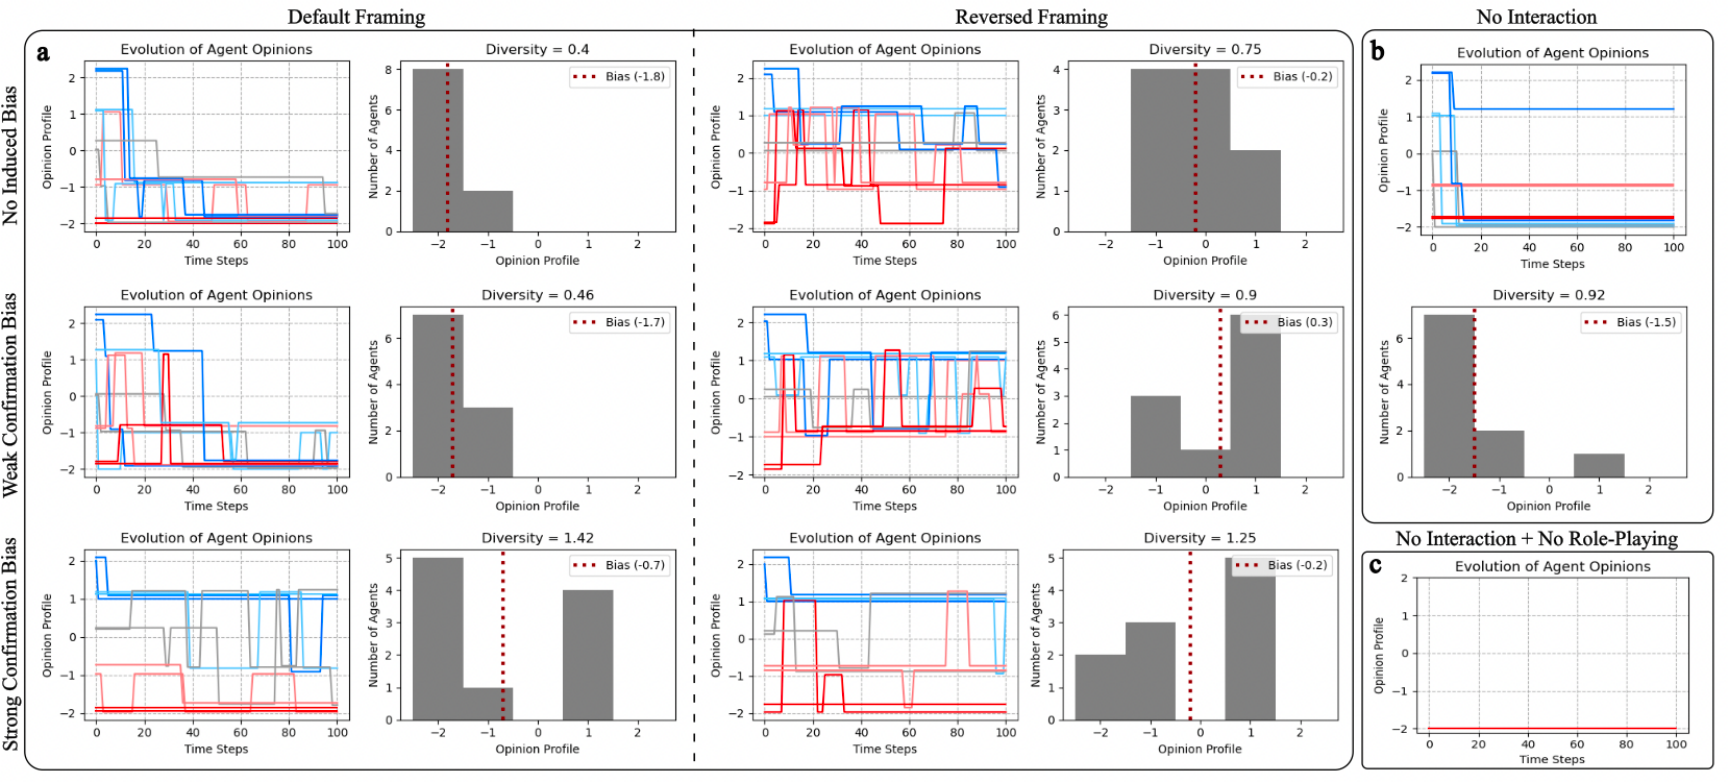}
\vspace{-2mm}
\caption{\textbf{Cumulative Memory:} Opinion trajectories $\langle o_i \rangle$ of LLM agents and the final opinion distribution $F_{o}^T$ for the topic of co-existence of T-Rex and humans across (a) different framings and cognitive biases, compared to baselines with (b) no interaction, and (c) no role-playing.}
\label{fig:trex_humans_cumulative}
\vspace{-4mm}
\end{figure*}
\begin{figure*}[htb!] 
\centering
\includegraphics[width=0.99\linewidth]{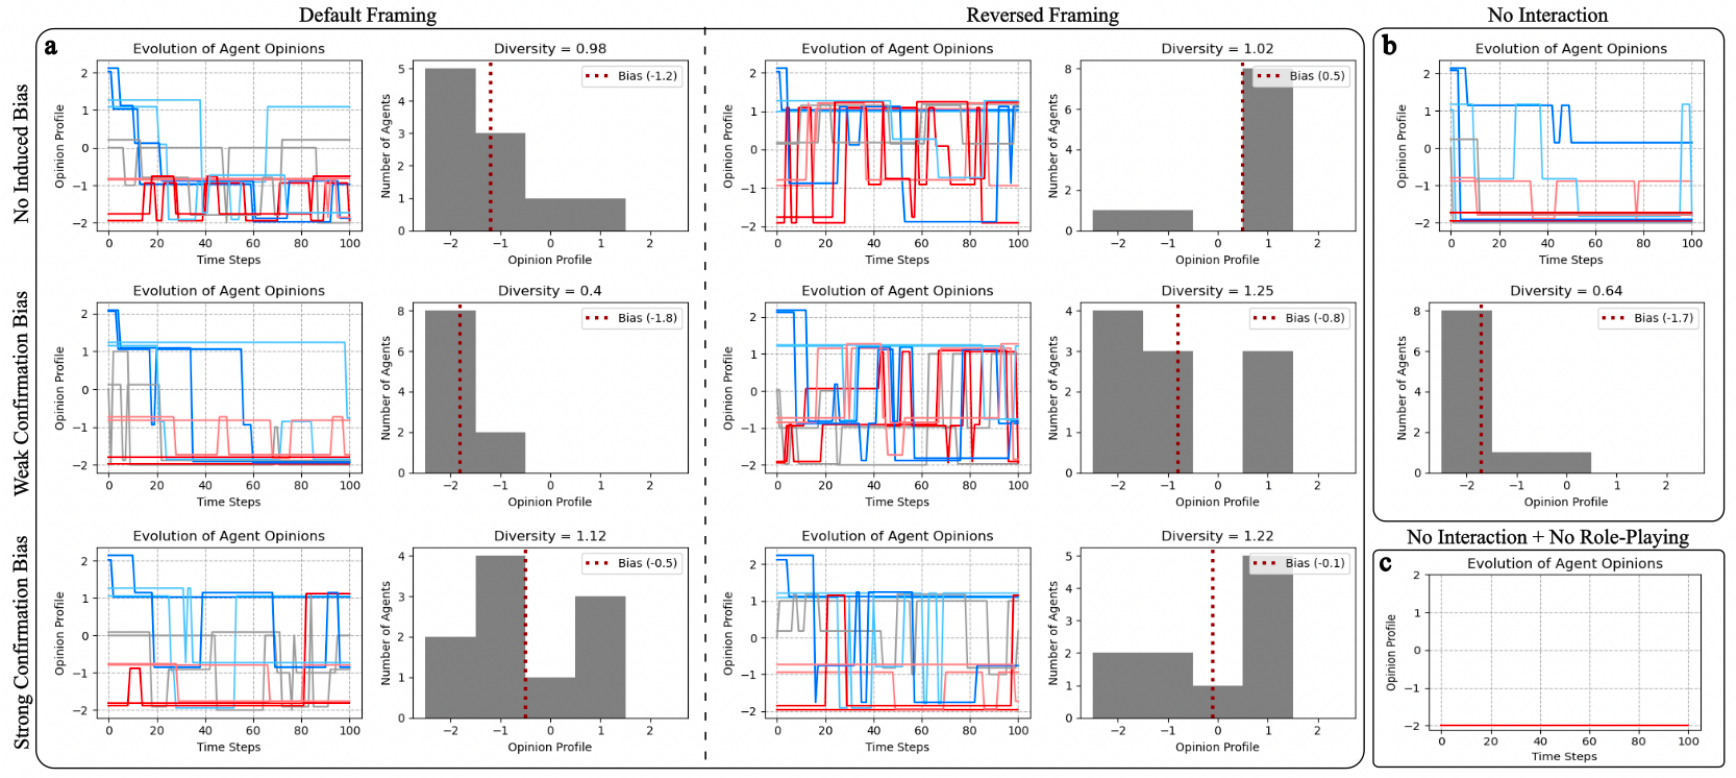}
\vspace{-2mm}
\caption{\textbf{Reflective Memory:} Opinion trajectories $\langle o_i \rangle$ of LLM agents and the final opinion distribution $F_{o}^T$ for the topic of co-existence of T-Rex and humans  across (a) different framings and cognitive biases, compared to baselines with (b) no interaction, and (c) no role-playing.}
\label{fig:trex_humans_reflective}
\vspace{-4mm}
\end{figure*}

\begin{figure*}[htb!] 
\centering
\includegraphics[width=0.99\linewidth]{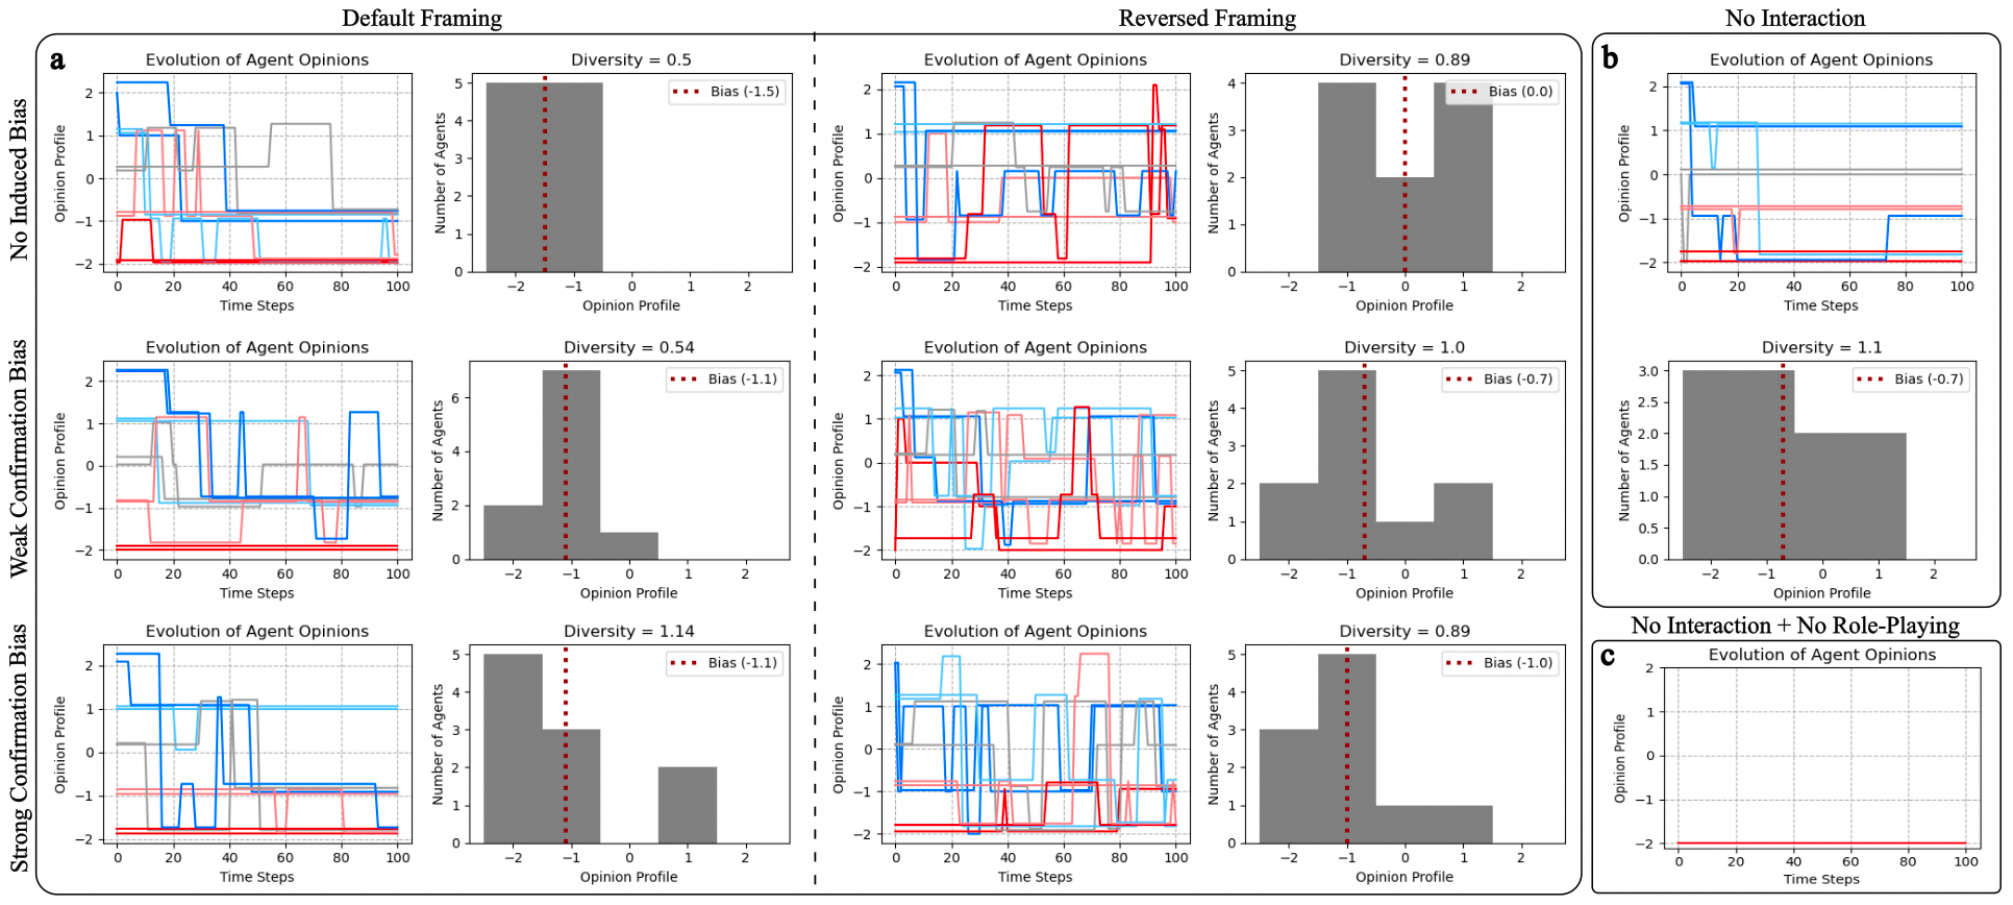}
\vspace{-2mm}
\caption{\textbf{Cumulative Memory:} Opinion trajectories $\langle o_i \rangle$ of LLM agents and the final opinion distribution $F_{o}^T$ for the topic of Talking to the Dead across (a) different framings and cognitive biases, compared to baselines with (b) no interaction, and (c) no role-playing.}
\label{fig:talking_to_dead_cumulative}
\vspace{-4mm}
\end{figure*}
\begin{figure*}[htb!] 
\centering
\includegraphics[width=0.99\linewidth]{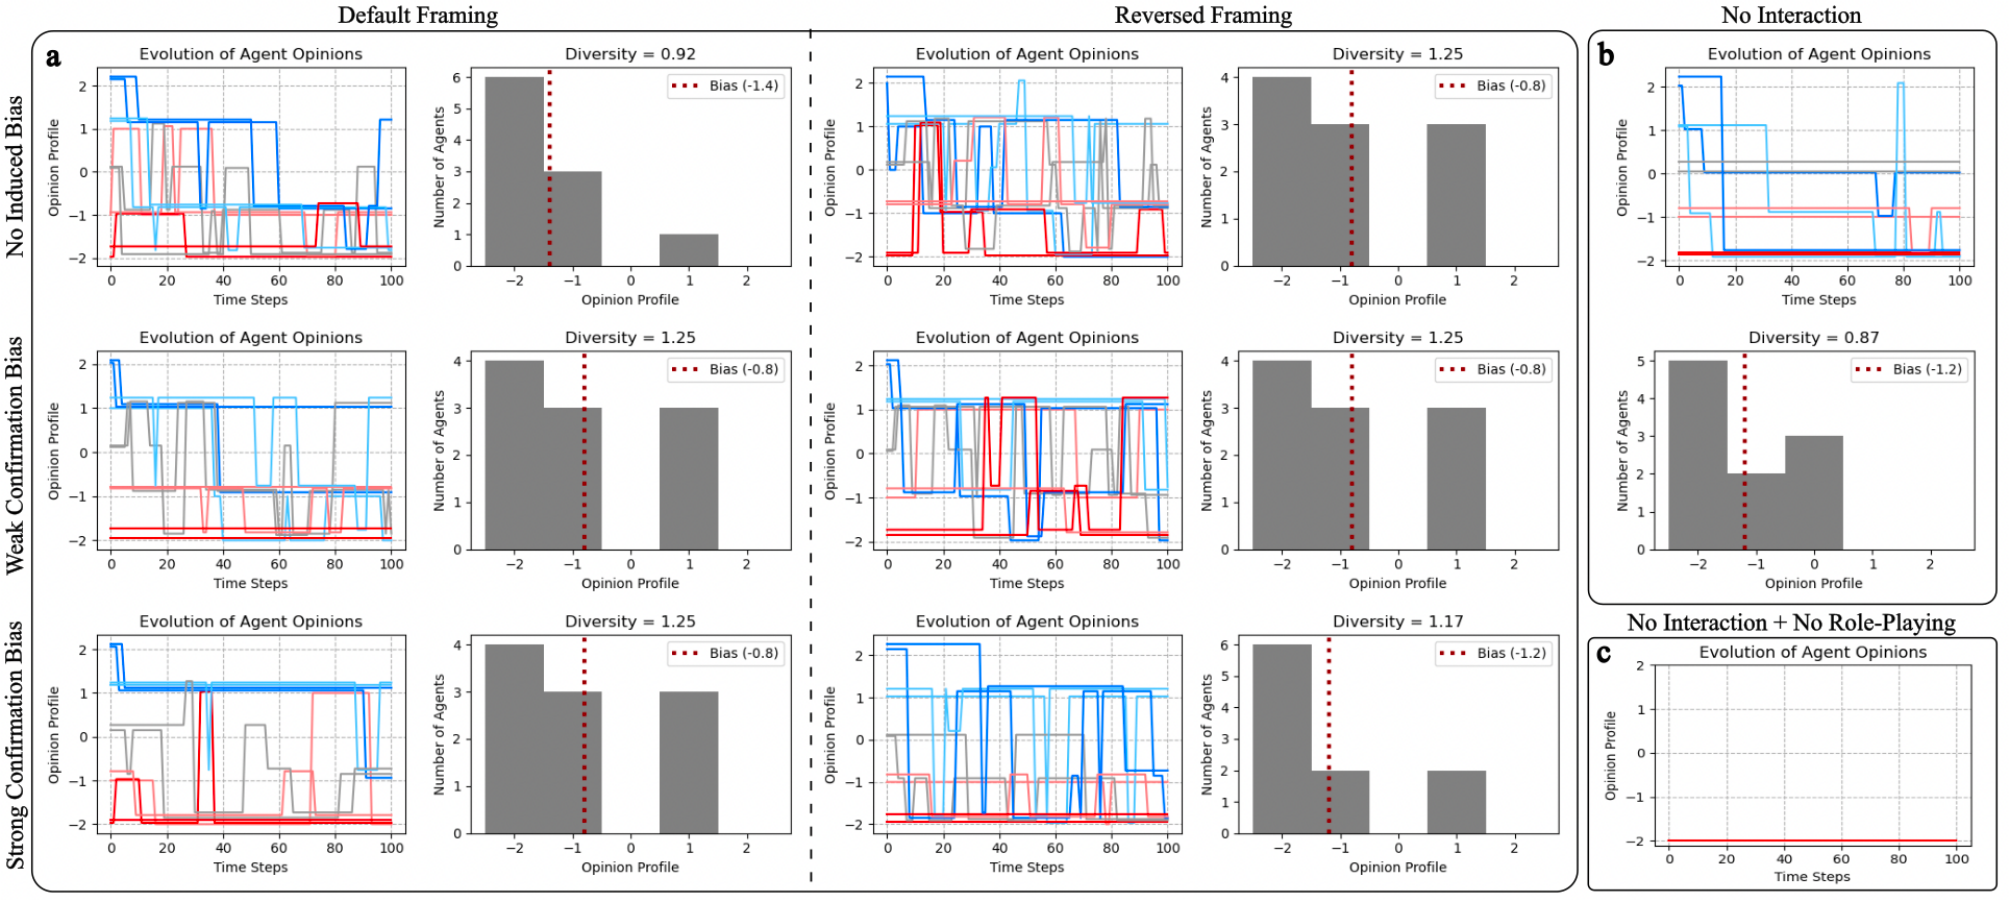}
\vspace{-2mm}
\caption{\textbf{Reflective Memory:} Opinion trajectories $\langle o_i \rangle$ of LLM agents and the final opinion distribution $F_{o}^T$ for the topic of Talking to the Dead across (a) different framings and cognitive biases, compared to baselines with (b) no interaction, and (c) no role-playing.}
\label{fig:talking_to_dead_reflective}
\vspace{-4mm}
\end{figure*}

\begin{figure*}[tb!] 
\centering
\includegraphics[width=0.99\linewidth]{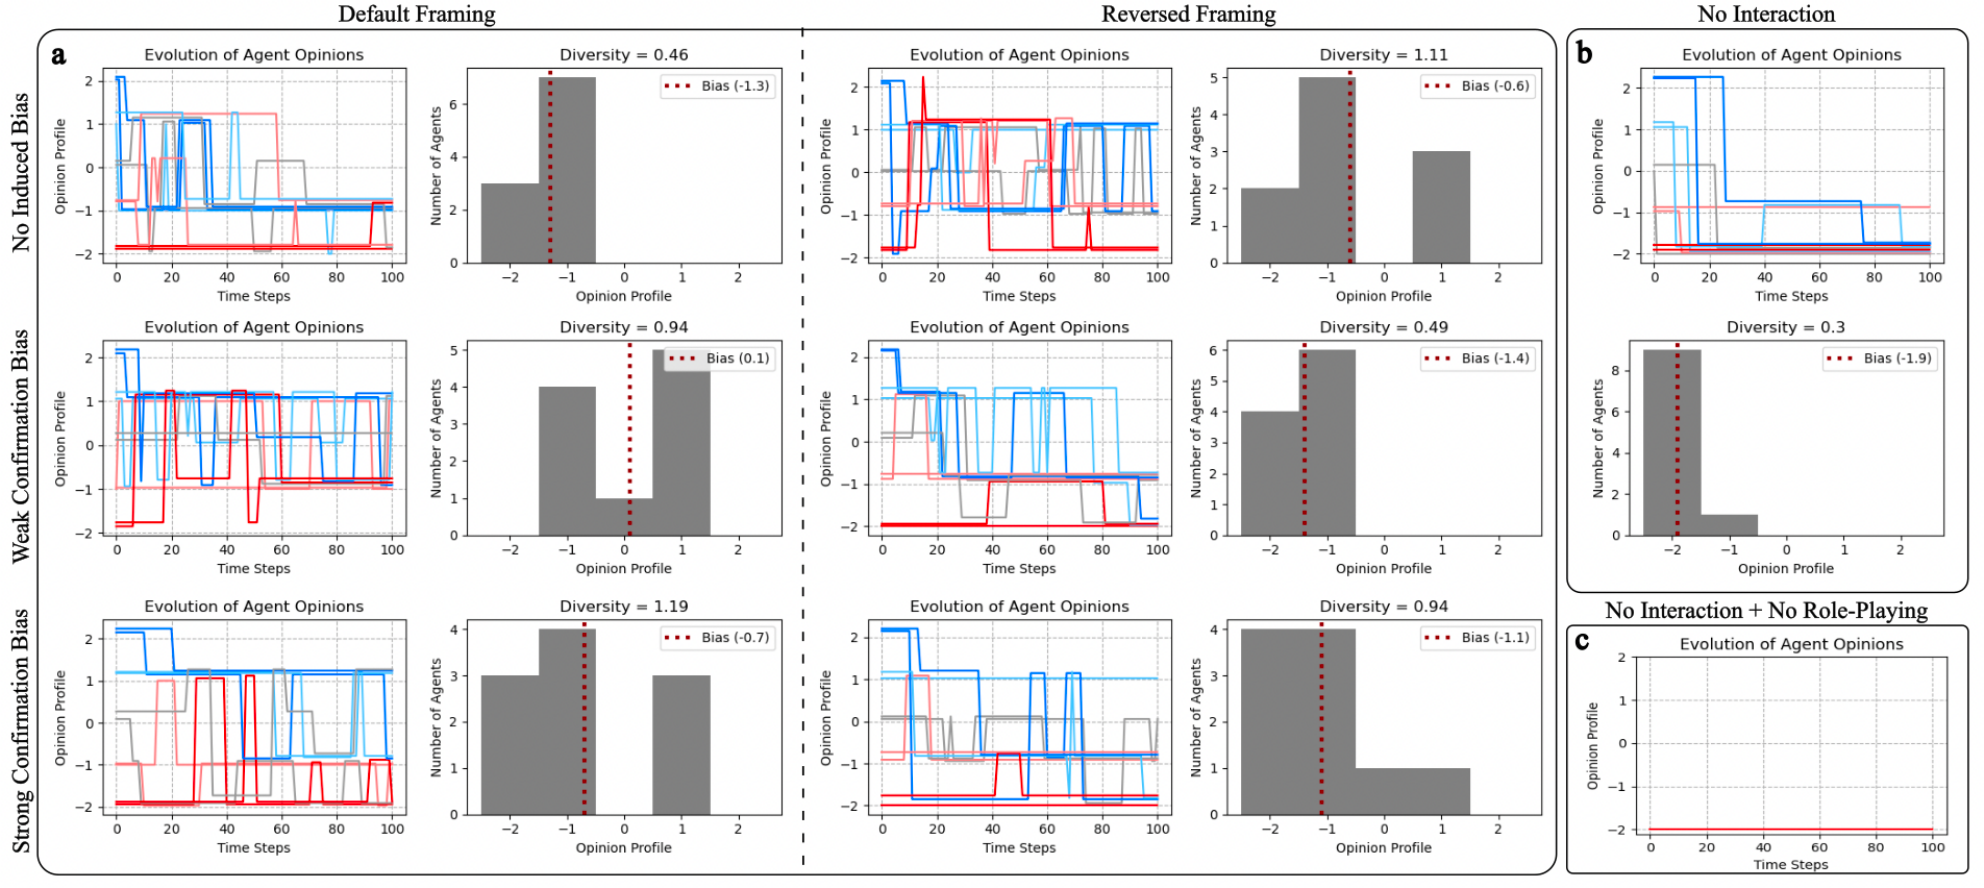}
\vspace{-2mm}
\caption{\textbf{Reflective Memory:} Opinion trajectories $\langle o_i \rangle$ of LLM agents  and the final opinion distribution $F_{o}^T$ for the topic of Predicting the Future by Palm Chracteristics across (a) different framings and cognitive biases, compared to baselines with (b) no interaction, and (c) no role-playing.}
\label{fig:future_predictions_cumulative}
\vspace{-4mm}
\end{figure*}
\begin{figure*}[tb!] 
\centering
\includegraphics[width=0.99\linewidth]{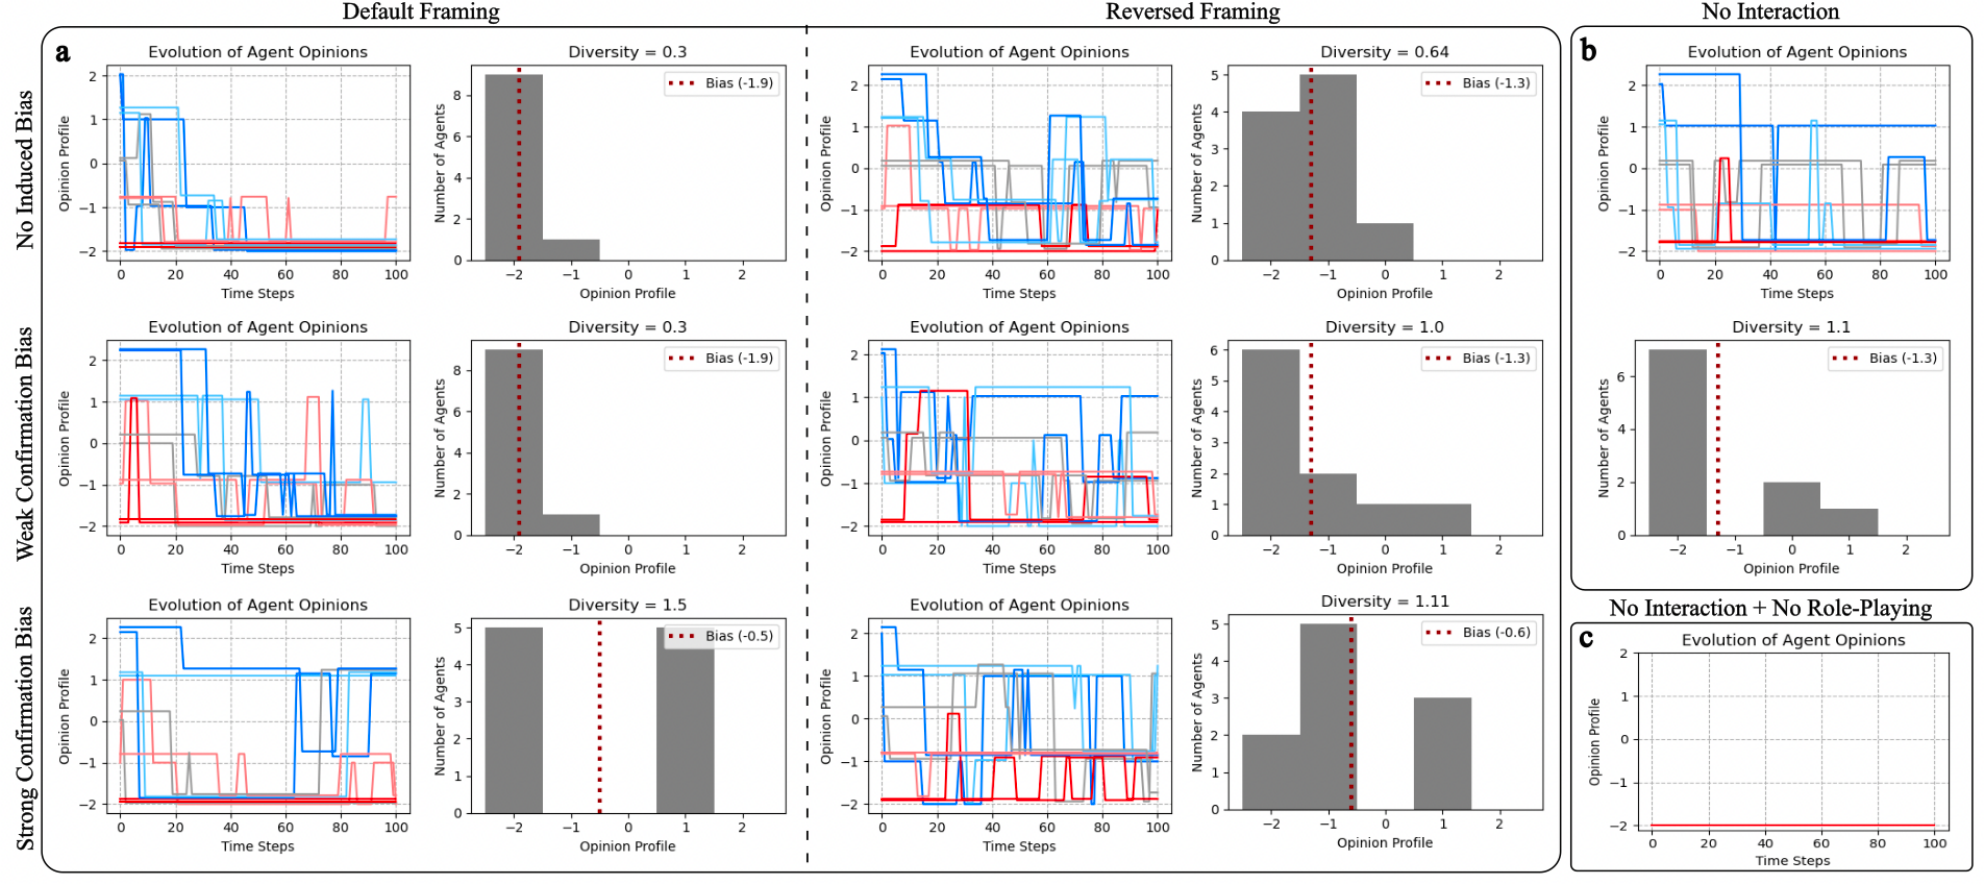}
\vspace{-2mm}
\caption{\textbf{Reflective Memory:} Opinion trajectories $\langle o_i \rangle$ of LLM agents  and the final opinion distribution $F_{o}^T$ for the topic of Predicting the Future by Palm Chracteristics across (a) different framings and cognitive biases, compared to baselines with (b) no interaction, and (c) no role-playing.}
\label{fig:future_predictions_reflective}
\vspace{-4mm}
\end{figure*}
