# Supplementary material for: Simulating Opinion Dynamics with Networks of LLM-based Agents
Source: arXiv:2311.09618 source file (2024-04-01)
Supplement: Supplementary file 2 [file result_per_topic_result_table.tex]

\section{Result Table of All Topics}\label{app:result_all_topics}

\begin{table*}[htb!]
\small
\centering
\begin{tabular}{@{}p{3cm}p{1cm}p{4cm}P{1.25cm}P{1.25cm}P{1.25cm}P{1.25cm}@{}}
\toprule
 &  && \multicolumn{2}{c}{\textbf{Cumulative Memory}} &  \multicolumn{2}{c}{\textbf{Reflective Memory}}\\
\toprule
\textbf{Topic}& \textbf{Framing} &\textbf{Cognitive Bias}&  \textbf{Bias} ($\textit{B}$)& \textbf{Diversity} ($\textit{D}$)& \textbf{Bias} ($\textit{B}$) & \textbf{Diversity} ($\textit{D}$)\\ \midrule
Flat Earth&  False&None& -2.0&  0.0&  -1.9&0.3\\
&  &Weak Confirmation Bias& -1.1&  1.22&  -1.4&0.92\\
&  &Strong Confirmation Bias& -1.3&  1.19&  -1.1&1.22\\
\cline{3-7}
&  True&None& 1.0&  0.0&  0.5&1.02\\
&  &Weak Confirmation Bias& -0.4&  1.2&  0.5&1.02\\
&   &Strong Confirmation Bias& -0.3&  1.35&  -1.1&1.37\\
\cline{2-7}
Global Warming&  False&None& -2.0&  0.0&  -1.6&0.66\\
\multicolumn{1}{@{\hspace{3em}}l}{} &  &Weak Confirmation Bias& -1.2&  1.08&  -0.6&1.56\\
\multicolumn{1}{@{\hspace{3em}}l}{} &  &Strong Confirmation Bias& -1.0&  1.34&  0.4&1.43\\
\cline{3-7}
 & True& None& 1.0& 0.0& 1.0&0.0\\
 & & Weak Confirmation Bias& 0.3& 1.1& 0.3&1.1\\
 & & Strong Confirmation Bias& -0.7& 0.9& -0.3&1.35\\
\cline{2-7}
 Predicting Future& False& None& -1.3& 0.46& -1.9&0.3\\
 & & Weak Confirmation Bias& 0.1& 0.94& -1.9&0.3\\
 & & Strong Confirmation Bias& -0.7& 1.19& -0.5&1.5\\
 \cline{3-7}
 & True& None& -0.6& 1.11& -1.3&0.64\\
 & & Weak Confirmation Bias& -1.4& 0.49& -1.3&1.0\\
 & & Strong Confirmation Bias& -1.1& 0.94& -0.6&1.11\\
\cline{2-7}
 Talk to the Dead& False& None& -1.5& 0.5& -1.4&0.92\\
 & & Weak Confirmation Bias& -1.1& 0.54& -0.8&1.25\\
 & & Strong Confirmation Bias& -1.1& 1.14& -0.8&1.25\\
 \cline{3-7}
 & True& None& 0.0& 0.89& -1.1&0.83\\
 & & Weak Confirmation Bias& -0.7& 1.0& -0.8&1.25\\
 & & Strong Confirmation Bias& -1.0& 0.89& -1.2&1.17\\
\cline{2-7}
 T-Rex and Humans& False& None& -1.8& 0.4& -1.2&0.98\\
 & & Weak Confirmation Bias& -1.7& 0.46& -1.8&0.4\\
 & & Strong Confirmation Bias& -0.7& 1.42& 0.5&1.02\\
 \cline{3-7}
 & True& None& -0.2& 0.75& -1.1&0.83\\
 & & Weak Confirmation Bias& 0.3& 0.9& -0.8&1.25\\
 & & Strong Confirmation Bias& -0.2& 1.25& -0.1&1.22\\
\bottomrule
\end{tabular}
\caption{\textbf{Topic-wise final state opinion dynamics analysis:} Presenting the Bias ($B$) and Diversity ($D$) metrics for both cumulative and reflective memory strategies under False and True framing conditions, and different levels of induced confirmation bias. \sn{TODO: add other topics}}
\label{tab:result_bias_diversity_per_topic}
\end{table*}

In this section, we report the result table (Table~\ref{tab:result_bias_diversity_per_topic}) for all 15 topics.
