# Supplementary material for: Simulating Opinion Dynamics with Networks of LLM-based Agents
Source: arXiv:2311.09618 source file (2024-04-01)
Supplement: Supplementary file 3 [file all_topic_table.tex]

\section{Detailed Final Opinion Profile Bias and Diversity for All Topics}\label{app:all_topics_table}

In Table \ref{tab:result_bias_diversity_per_topic}, we report the bias ($\mathbf{B}$) and diversity ($\mathbf{D}$) metrics for all different topics of debates, with both false and true topic framing, different levels of induced confirmation bias, and two memory implementations.
