# Supplementary material for: Simulating Opinion Dynamics with Networks of LLM-based Agents
Source: arXiv:2311.09618 source file (2024-04-01)
Supplement: Supplementary file 4 [file skewed_flat_earth.tex]

\section{Results for Skewed Initial Distribution for Debate on Flat Earth}\label{app:result_skewed_flat_earth}

In this section, we report results of altering the initial opinion distribution of the agents to be all positive or all negative or skewed towards the positive or negative side on the topic of debate of a flat-earth. As seen in \Scref{subsec:initial_opinion_distribution}, we see a very strong bias of the agents to converge to the truth, irrespective of their initial opinion distribution.
\begin{figure*}[tb!] 
\centering
\includegraphics[width=0.99\linewidth]{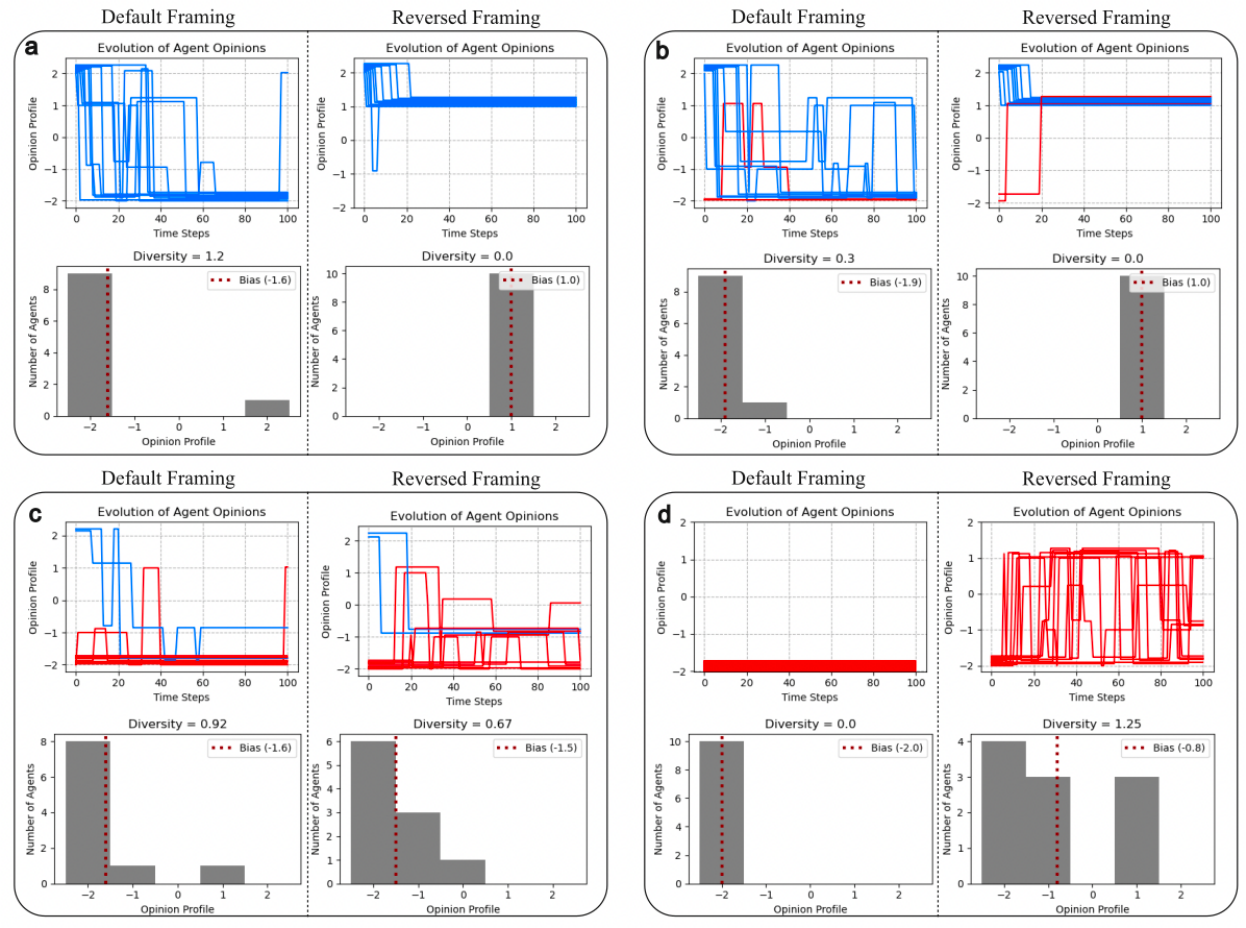}
\vspace{-2mm}
\caption{Skewed opinion distribution for flat earth debate. (Panel \textbf{a}) All agents start with a strongly positive opinion (Panel \textbf{b}) $8$ agents start with a strongly positive opinion while $2$ with a strongly negative opinion (Panel \textbf{c}) $8$ agents start with a strongly negative opinion while $2$ with a strongly positive opinion. (Panel \textbf{d}) All agents start with a strongly negative opinion.}
\label{fig:skewed_flat_earth}
\vspace{-4mm}
\end{figure*}
